# Supplementary material for: R-MBO: A Multi-surrogate Approach for Preference Incorporation in Multi-objective Bayesian Optimisation
Source: arXiv:2204.13166 source file (2022-04-27)
Supplement: Supplementary file 1 [file Preference_Incorporation_BO_Supplementary_arXiv.pdf]

# Supplementary Material

## R-MBO: A Multi-surrogate Approach for Preference Incorporation in Multi-objective Bayesian Optimisation

Tinkle Chugh

t.chugh@exeter.ac.uk

Department of Computer Science

University of Exeter

Exeter, United Kingdom

### 1 LAPLACE APPROXIMATION CALCULATIONS FOR BI-OBJECTIVE OPTIMISATION

Let us denote  $mi = w_i(\mu_i - z_i^*)$  and  $si = w_i\sigma_i$ , where  $\mu_i$ ,  $\sigma_i$ ,  $z_i^*$  and  $w_i$  are the  $i^{th}$  element of the posterior mean vector, the standard deviation vector, the desirable objective vector and the weight vector, respectively. The distribution of  $g$  can also be written as:

$$p(g) = \frac{1}{4} \text{Erfc} \left[ \frac{-g-m1}{\sqrt{2}s1} \right] \left( \frac{e^{-\frac{(g-m1)^2}{2s1^2}} \sqrt{\frac{2}{\pi}}}{s1 \text{Erfc} \left[ \frac{-g-m1}{\sqrt{2}s1} \right]} + \frac{e^{-\frac{(g-m2)^2}{2s2^2}} \sqrt{\frac{2}{\pi}}}{s2 \text{Erfc} \left[ \frac{-g-m2}{\sqrt{2}s2} \right]} \right) \text{Erfc} \left[ \frac{-g-m2}{\sqrt{2}s2} \right] \quad (1)$$

The mode,  $g_0$  can be calculated by taking the derivative of the  $\log g$  i.e.  $\frac{d \log g}{dg} = 0$ :

$$\frac{4s1^2s2^2 + \sqrt{2}\pi \left( -e^{-\frac{(g-m1)^2}{2s1^2}} (g-m2)s1^3 \text{Erfc} \left[ \frac{-g+m1}{\sqrt{2}s1} \right] - e^{-\frac{(g-m2)^2}{2s2^2}} (g-m1)s2^3 \text{Erfc} \left[ \frac{-g+m2}{\sqrt{2}s2} \right] \right)}{\sqrt{2}\pi s1^2s2^2 \left( e^{-\frac{(g-m1)^2}{2s1^2}} s1 \text{Erfc} \left[ \frac{-g+m1}{\sqrt{2}s1} \right] + e^{-\frac{(g-m2)^2}{2s2^2}} s2 \text{Erfc} \left[ \frac{-g+m2}{\sqrt{2}s2} \right] \right)} = 0 \quad (2)$$

The equation does not have a closed form expression for estimating the mode. Therefore, the mode can be estimated by maximising a posteriori with an iterative method e.g. Newton's method.

Once the mode is known, we can estimate the second derivative at the mode:

$$\begin{aligned} & A \\ & = - \left( \frac{d^2 \log g}{dg^2} \right)_{g=g_0} \\ & = \left( -e^{-\frac{(g-m1)^2}{2s1^2}} \pi s1^5 s2 \text{Erfc} \left[ \frac{-g+m1}{\sqrt{2}s1} \right]^2 \right. \\ & \quad + e^{-\frac{(g-m1)^2}{2s1^2}} \text{Erfc} \left[ \frac{-g+m1}{\sqrt{2}s1} \right] \\ & \quad \left( \sqrt{2}\pi s1^2s2 \left( (g-m2)s1^2 + 3(-g+m1)s2^2 \right) \right. \\ & \quad + e^{-\frac{(g-m2)^2}{2s2^2}} \pi \left( (g-m2)^2s1^4 - s1^2 \left( 2(g-m1)(g-m2) + s1^2 \right) s2^2 + (g-m1-s1)(g-m1+s1)s2^4 \right) \\ & \quad \left. \left. \text{Erfc} \left[ \frac{-g+m2}{\sqrt{2}s2} \right] \right) \right. \\ & \quad - s1s2^2 \left( 8s1^2s2 + e^{-\frac{(g-m2)^2}{2s2^2}} \sqrt{2}\pi \left( 3(g-m2)s1^2 + (-g+m1)s2^2 \right) \right. \\ & \quad \left. \left. \text{Erfc} \left[ \frac{-g+m2}{\sqrt{2}s2} \right] \right) \right. \\ & \quad \left. + e^{-\frac{(g-m2)^2}{2s2^2}} \pi s2^3 \text{Erfc} \left[ \frac{-g+m2}{\sqrt{2}s2} \right]^2 \right) \right) \quad (3) \\ & = \left( \pi s1^3s2^3 \left( e^{-\frac{(g-m1)^2}{2s1^2}} s1 \text{Erfc} \left[ \frac{-g+m1}{\sqrt{2}s1} \right] \right. \right. \\ & \quad \left. \left. + e^{-\frac{(g-m2)^2}{2s2^2}} s2 \text{Erfc} \left[ \frac{-g+m2}{\sqrt{2}s2} \right] \right)^2 \right) \end{aligned}$$

After estimating the mode and the second derivative at the mode, the distribution of  $g$  can be written as:

$$g \sim \mathcal{N}(g_0, A^{-1}),$$

where  $g_0$  is the mean and  $A^{-1}$  is the variance. These calculations allow us to use the closed form expression of acquisition functions e.g. expected improvement and probability of improvement.

### 2 NUMERICAL EXPERIMENTS

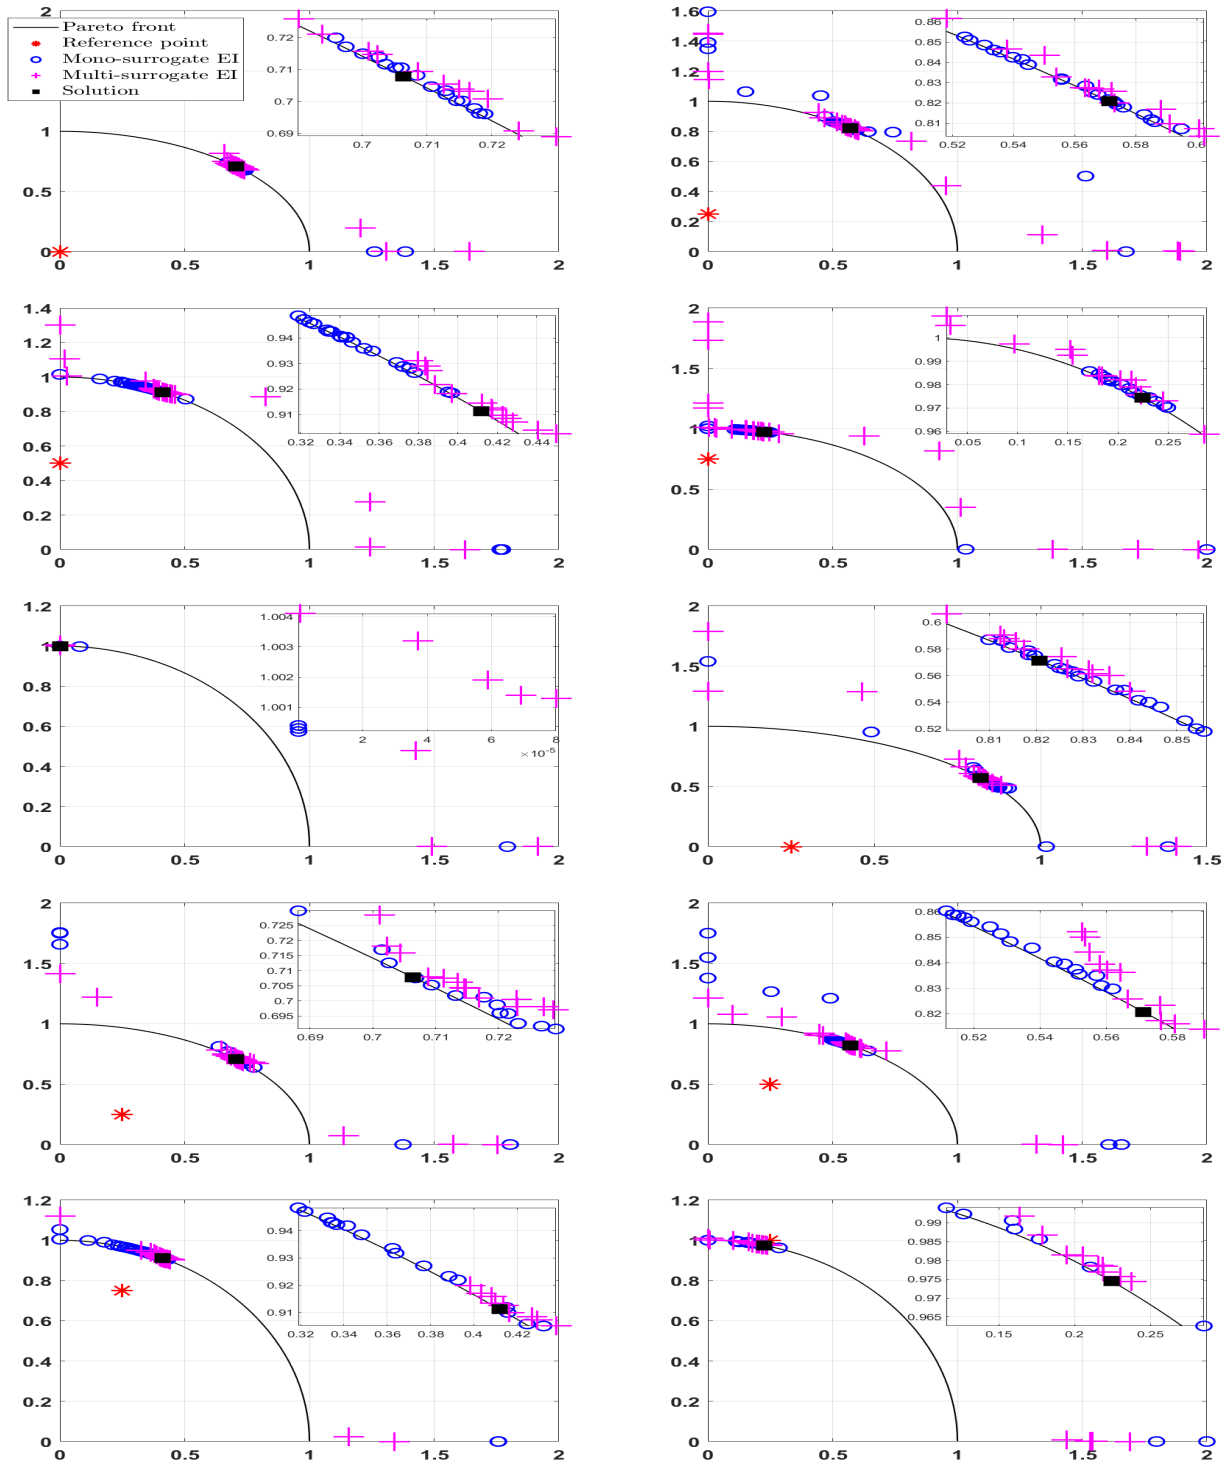

Figure 1: Performance on DTLZ2

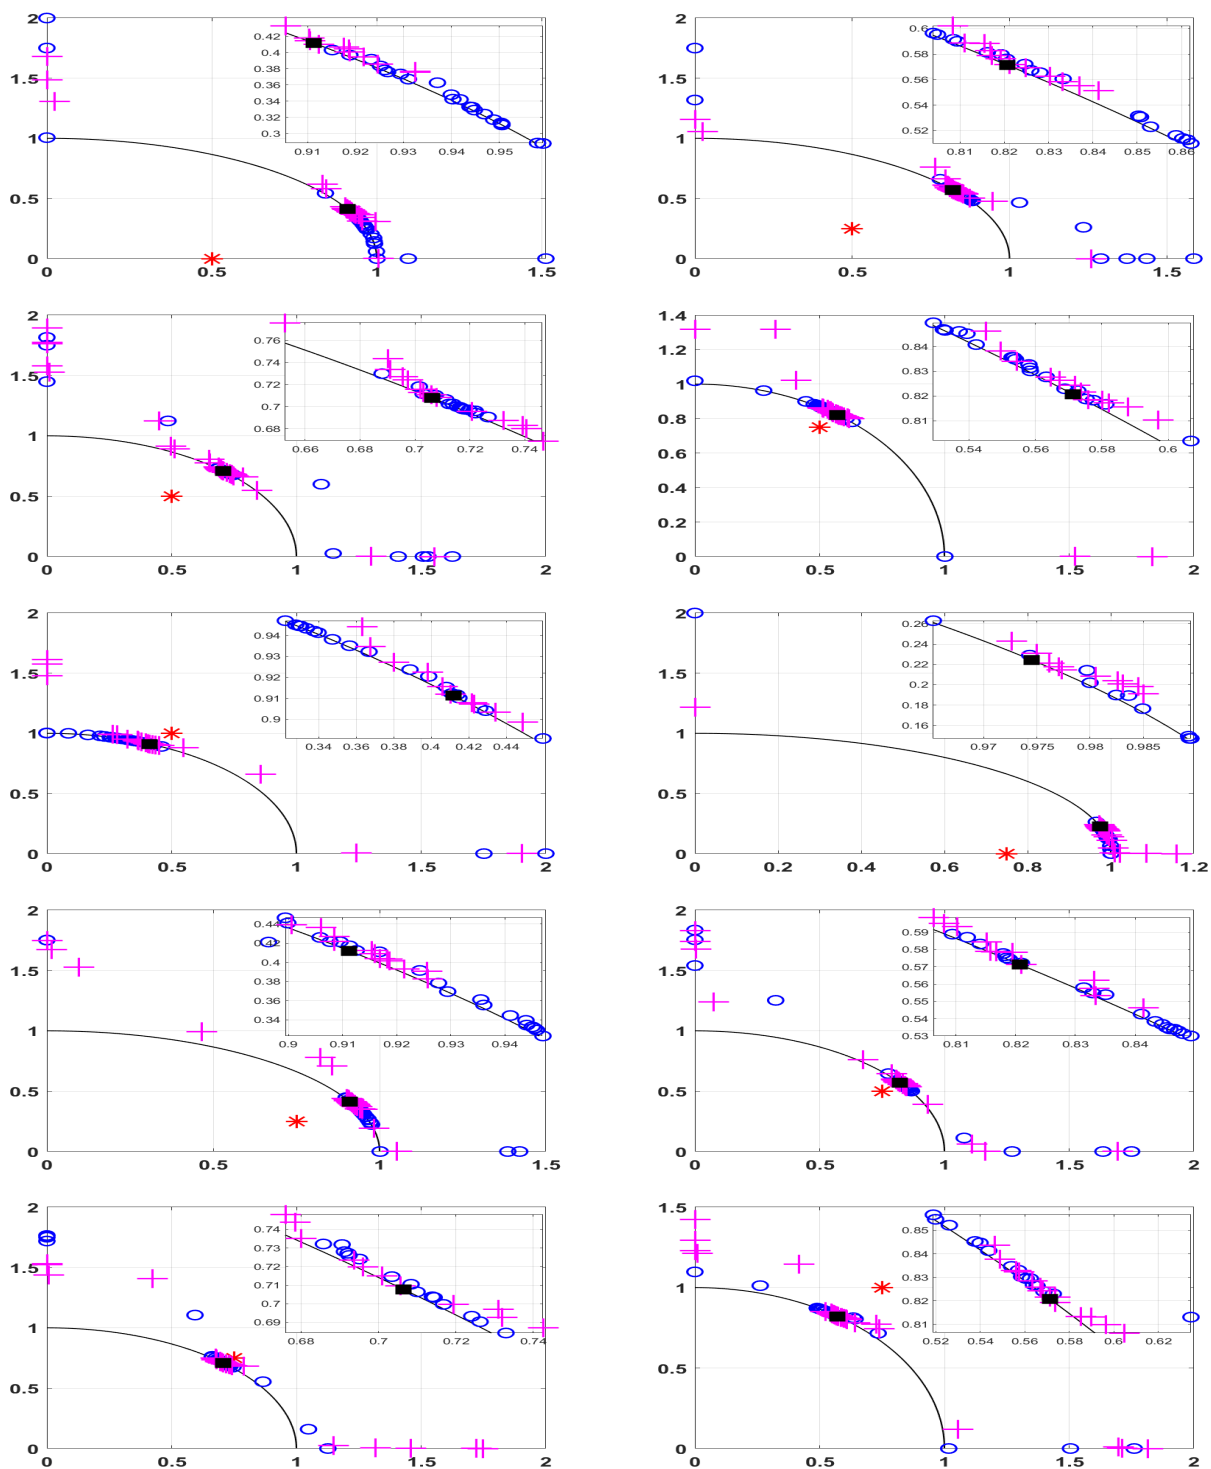

Figure 2: Performance on DTLZ2

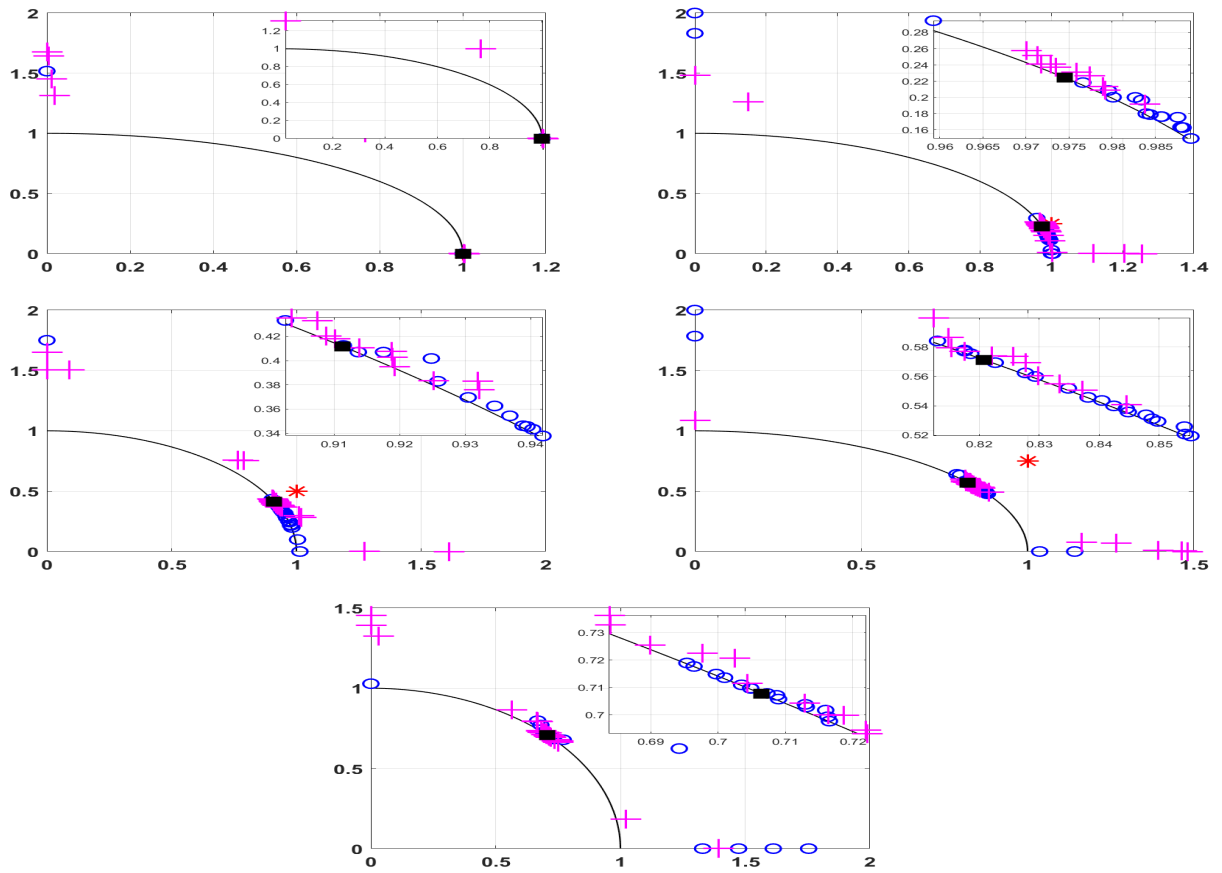

Figure 3: Performance on DTLZ2

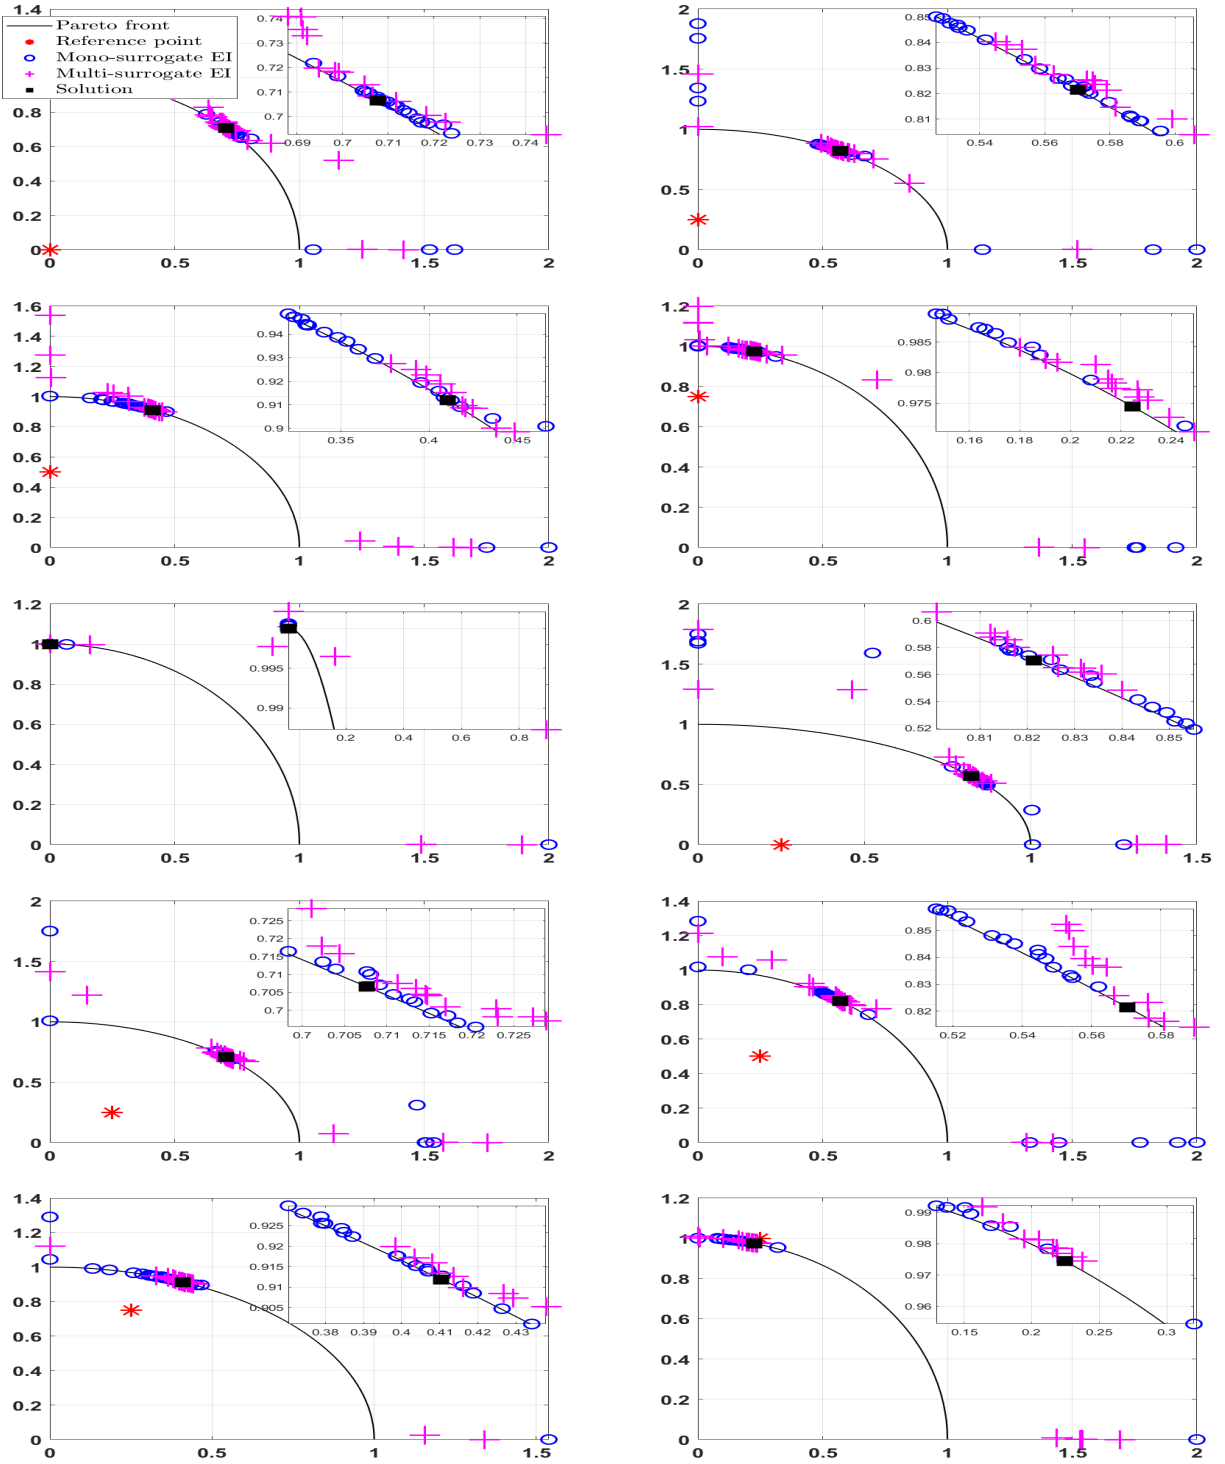

Figure 4: Performance on DTLZ5

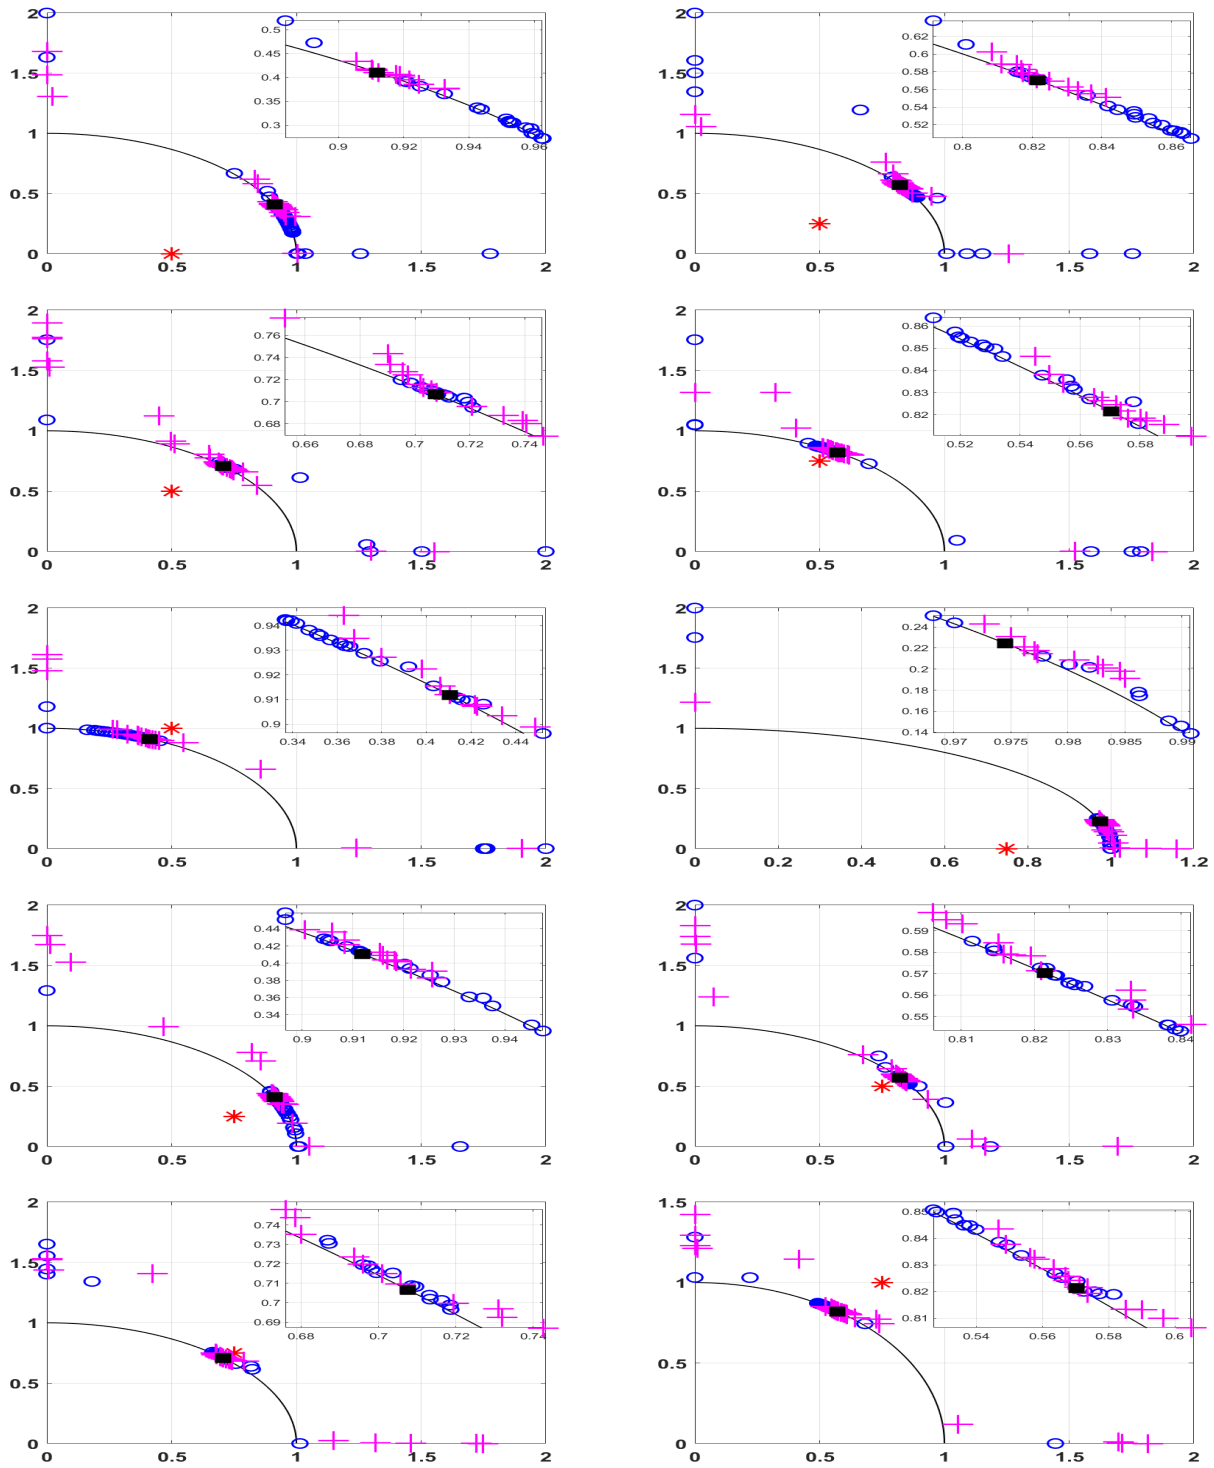

Figure 5: Performance on DTLZ5

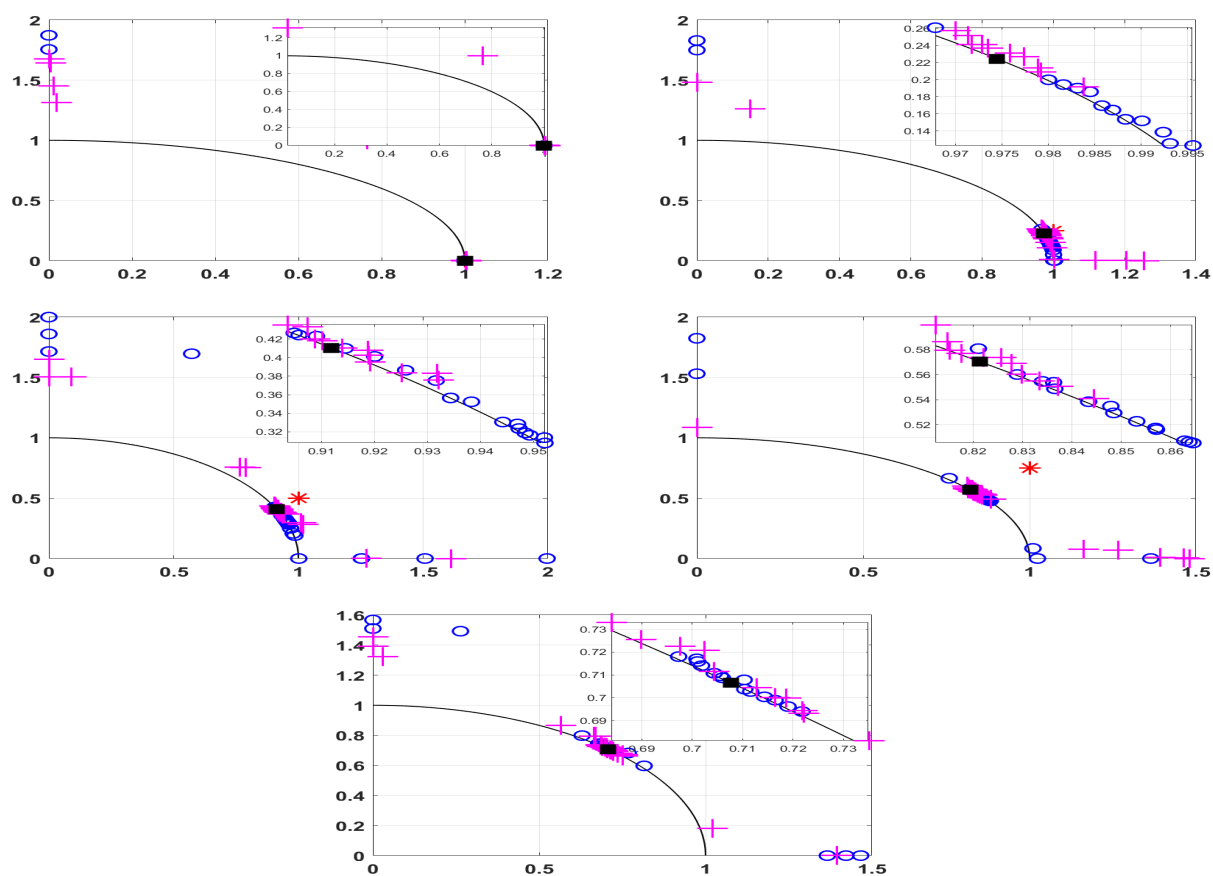

Figure 6: Performance on DTLZ5

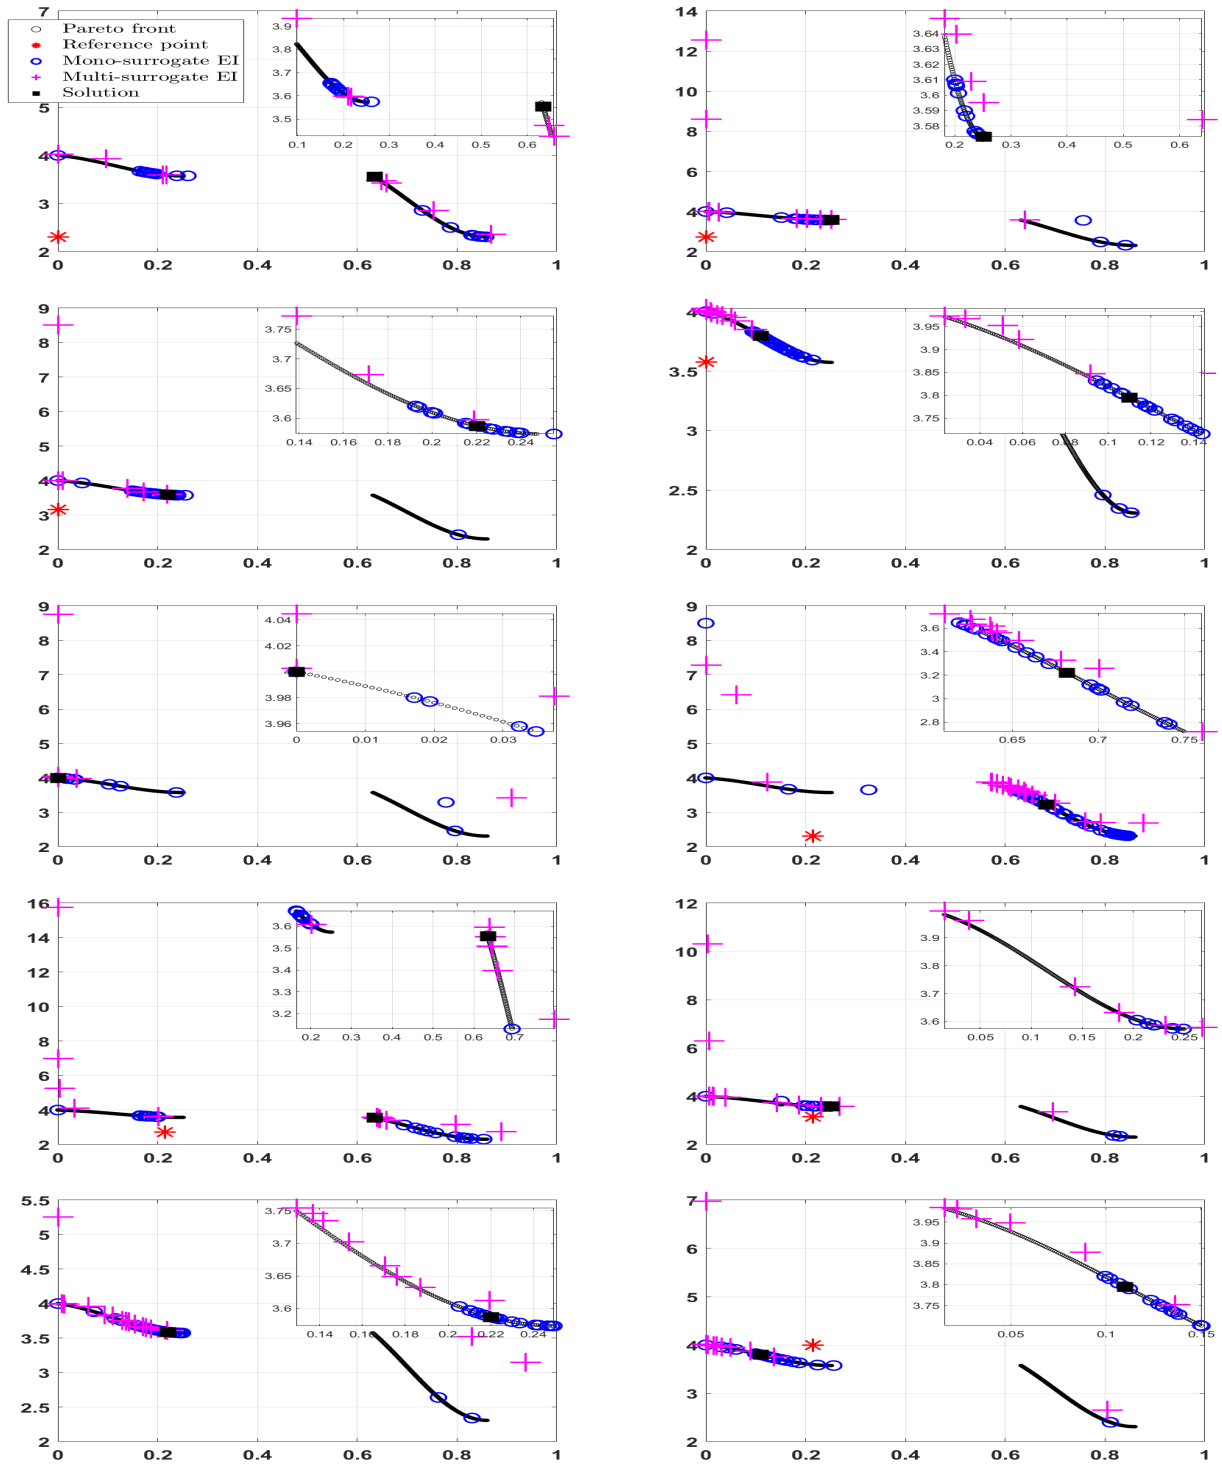

Figure 7: Performance on DTLZ7

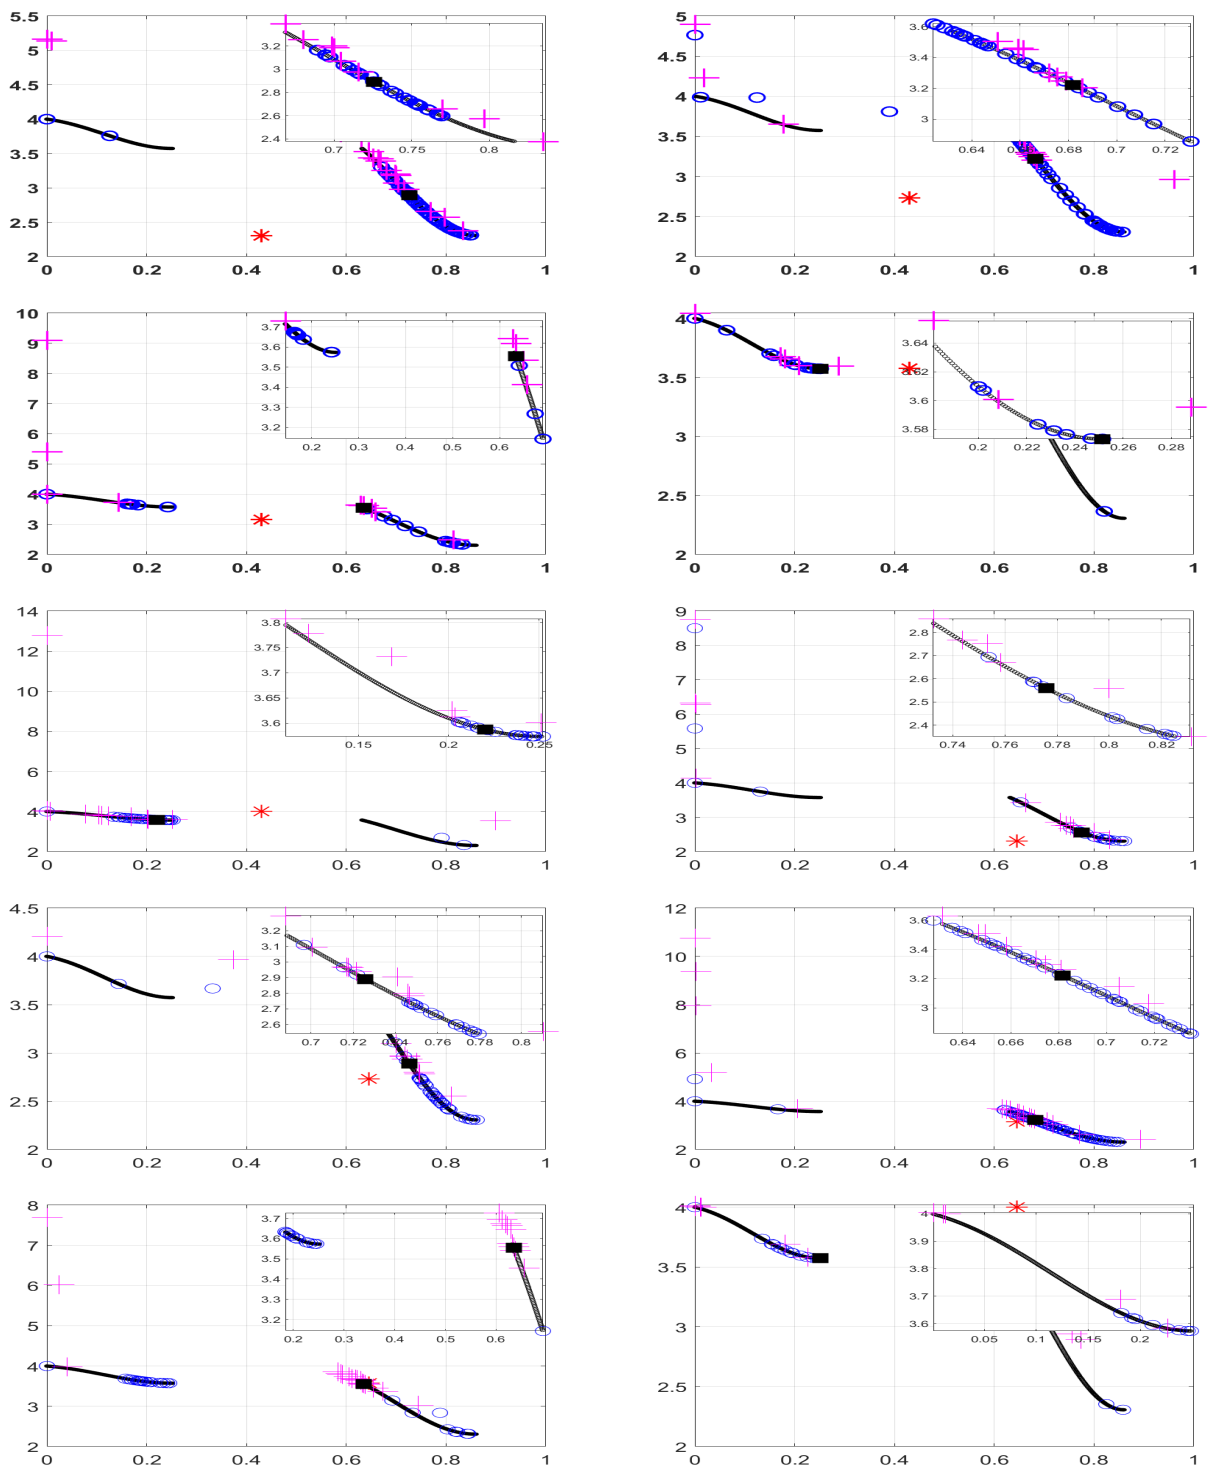

Figure 8: Performance on DTLZ7

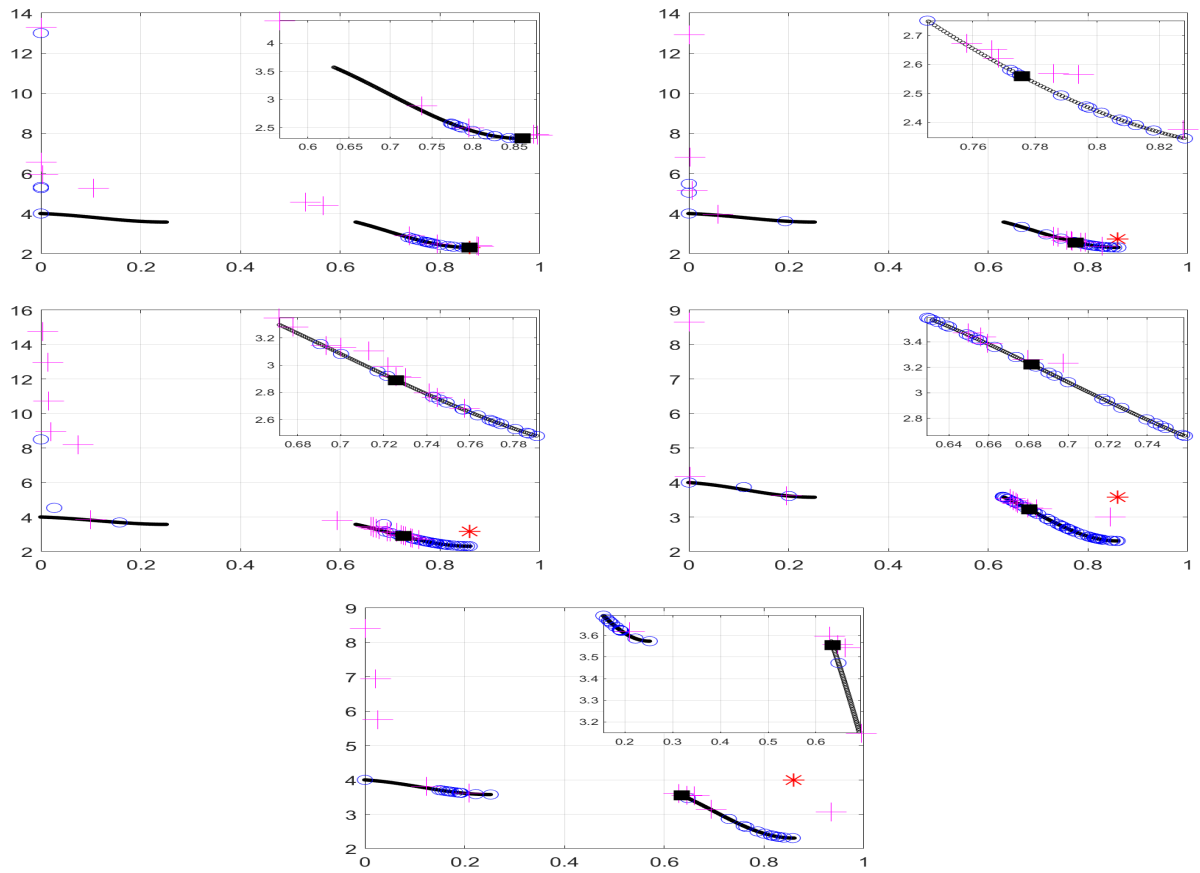

Figure 9: Performance on DTLZ7
